# Supplementary material for: EasyCrash: Exploring Non-Volatility of Non-Volatile Memory for High Performance Computing Under Failures
Source: arXiv:1906.10081 source file (2019-06-24)
Supplement: Supplementary file 1 [file appendixA.tex]

\section{Benchmark Information}
